# Supplementary material for: Universality in the emergence of oscillatory instabilities in turbulent flows
Source: arXiv:1910.05802 source file (2019-10-13)
Supplement: Supplementary file 1 [file Supplementary.pdf]

# Universality in the emergence of oscillatory instabilities in turbulent flows (supplementary information)

Induja Pavithran[1], Vishnu R. Unni[2], Alan J. Varghese[3], R. I. Sujith[3], Abhishek Saha[2], Norbert Marwan[4] and Jürgen Kurths[4,5,6]

[1] *Department of Physics, IIT Madras, Chennai-600036, India*
[2] *Department of Mechanical and Aerospace Engineering, University of California, San Diego, USA*
[3] *Department of Aerospace Engineering, IIT Madras, Chennai-600036, India*
[4] *Potsdam Institute for Climate Impact Research, Germany*
[5] *Department of Physics, Humboldt University, Germany*
[6] *Institute for Complex Systems and Mathematical Biology, University of Aberdeen, United Kingdom*

PACS 43.28.Kt – Aerothermoacoustics and combustion acoustics
PACS 47.20.-k – Flow instabilities
PACS 47.53.+n – Fractals in fluid dynamics

**Abstract** –*** Missing author ***

**Appendixes.** –

**Appendix A: Estimation of Hurst exponent.** – There are several algorithms for calculating the Hurst exponent ($H$). They include multifractal detrended fluctuation analysis (MFDFA) [1], rescaled range analysis ($R/S$) [2], wavelet approach [1], and multifractal detrended moving average (MFDMA) [3]. Among these techniques, we use MFDFA [1,4].

For a given time series $x(t)$ of length $N$, the mean subtracted cumulative deviate series $Y(k)$ is defined as,

$$Y(k) = \sum_{t=1}^{k} [x_t - < x >], \qquad k = 1, 2, ..., N, \tag{1}$$

where $< x >$ is the mean of the time series. We first divide the deviate series $Y(k)$ into $N_w = [N/w]$ non-overlapping segments of equal length $w$, where $[N/w]$ represents the greatest integer function. Then, we calculate the local trend for each of these segments $i$ by a polynomial fit of the series and obtain the fluctuations by subtracting the polynomial fit ($\bar{Y_i}$) from the deviate series ($Y_i$). The polynomial fit we use in the current study is of order 1. The variance of fluctuations is determined as,

$$F^2(w,i) = \frac{1}{w}\Big[\sum_{t=1}^{w} (Y_i(t) - \bar{Y_i})^2\Big], \tag{2}$$

for each segment $i = 1, 2, ..., N_w$.

The structure function of order 2 and span $w$, $F_w^2$ can be obtained as follows:

$$F_w^2 = \Big[\frac{1}{N_w}\sum_{i=1}^{N_w} F^2(w,i)\Big]^{1/2}. \tag{3}$$

We repeat the above steps for different time scales or span $w$. The slope of the linear regime in a log-log plot of $F_w^2$, for a range of span sizes $w$ gives the Hurst exponent ($H$).

$H$ represents the scaling of the *rms* of the standard deviation of fluctuations with the scale size or the time interval considered for obtaining the fluctuations. It provides a measure of persistence in a time series, *i.e.*, $H$ quantifies the information about the memory retained by the system. Generally, the $H$ has values between 0 and 1 for time series of fractal dimension between 1 and 2. The fractal dimension ($D$) and the Hurst exponent are related as $D = 2 - H$ in the case of a time series. For an antipersistent time series, $H < 0.5$ and $H > 0.5$ represents a persistent time series in which subsequent values are highly correlated. $H$ = 0.5 corresponds to an uncorrelated random process.

In our analysis, we compute $H$ for the time series corresponding to the unsteady variable obtained at each state during the transition to oscillatory instability in thermoacoustic, aeroacoustic and aeroelastic systems. $H$ for each state is calculated from the time series segments of selected duration. The choice of the range of segment length

should be optimal to capture the transition from an aperiodic state to a periodic state [5]. The periodicity at the onset of oscillatory instability will not be captured if we select segments of the length corresponding to less than one cycle of oscillation. Further, the fluctuations will be averaged out if we choose segments larger than four cycles. Therefore, two to four cycles of oscillations during the periodic regime is optimal for getting reliable results.

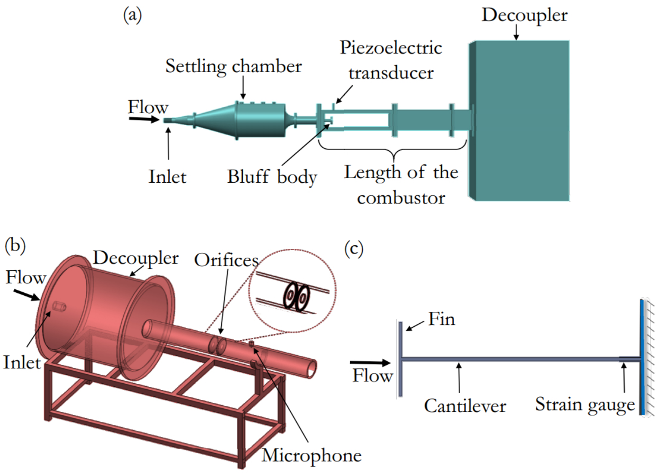


Fig. S1: Schematic of the experimental setups. (a) Turbulent combustor (thermoacoustic system) exhibiting transition to thermoacoustic instability. Mass flow rate of air is increased by keeping the mass flow rate of fuel constant thus increasing *Re* to attain different dynamical states. The acoustic pressure fluctuations are acquired using a piezoelectric transducer. (b) An aeroacoustic system with two orifices. Vortices are shed when the turbulent flow passes through the orifices. We increase the mass flow rate of the air to achieve different dynamical states. We measure the acoustic pressure fluctuations during the transition to aeroacoustic instability. (c) In the aeroelastic system, the left end of the beam has a small vertical fin attached to it, akin to a winglet of an aircraft wing. When a jet of air passes along the length of the cantilever from left to right, vortices are shed from the fins. These vortices impart an unsteady aerodynamic load to the cantilever. We measure the resulting strain on the cantilever close to the fixed end of the beam. The control parameter in this case is the mean velocity of the jet.

**Appendix B: Experiments.** – We analyze data from thermoacoustic, aeroacoustic and aeroelastic systems to study the transition from chaos to oscillatory instabilities by changing the respective control parameters.

*Experiments on Thermoacoustic system.* The thermoacoustic data analyzed in this study are reported in Nair & Sujith [6], Nair *et al.* [7] and Unni & Sujith [8]. The schematic of the experimental setup is shown in Fig. S1a and detailed descriptions can be found in these references. The length of the combustion chamber is varied to achieve different acoustic length scales and timescales. Also, the combustor can be equipped with different flame stabilization mechanisms. In this present work, data is presented for a bluff-body stabilized combustor for two lengths: 700 mm and 1400 mm. As opposed to this configuration, we also present data for a swirl stabilized combustor of length 700 mm. The different flame stabilizing mechanisms renders completely different flow physics in the combustor leading to different mechanisms causing thermoacoustic instability [9, 10]. Liquified petroleum gas (LPG: butane 60% and propane 40% composition by mass) is used as the fuel. Air is partially premixed with LPG before the reactant mixture enters the combustion chamber. The equivalence ratio is defined as $\phi = \frac{(\dot{m}_f/\dot{m}_a)_{actual}}{(\dot{m}_f/\dot{m}_a)_{stoichiometry}}$, where $\dot{m}_f$ and $\dot{m}_a$ are the mass flow rates of fuel and air, respectively. Mass flow rate of air is increased by keeping the mass flow rate of fuel constant. As the equivalence ratio is decreased, the system attains different dynamical states. The mass flows rates of air and fuel are controlled using mass flow controllers (Alicat MCR series) with an uncertainty of $\pm$ (0.8% of reading + 0.2% of full scale). The details of the procedure for the estimation of *Re* can be found in Nair & Sujith [6].

The Strouhal number is calculated as $S_t = fl/u$, where $f$ is the frequency of dominant mode of oscillations, $l$ is the characteristic length and $u$ is the velocity. We take the step size of the combustor as $l$. For the bluff body stabilized combustor of length 700 mm, $f$ is $\sim$250 Hz and the $S_t$ varies from 0.919 $\pm$ 0.016 to 0.58 $\pm$ 0.008. $f$ for bluff body stabilized combustor of length 1400 mm is $\sim$120 Hz and $S_t$ varies from 0.0.269 $\pm$ 0.005 to 0.223 $\pm$ 0.003. For swirl stabilized combustor (length 700 mm), $f$ is $\sim$250 Hz and $S_t$ varies from 0.876 $\pm$ 0.015 to 0.711 $\pm$ 0.011. The unsteady pressure fluctuations inside the combustion chamber are measured using piezoelectric transducers. PCB106B50 transducer (sensitivity 72.5 mV/kPa and resolution 0.48 Pa) is used for the combustor with 700 mm length and PCB103B02 (sensitivity 217.5 mV/kPa and resolution 0.15 Pa) transducer is used for the combustor with length 1400 mm. The sensor is located at the antinode of pressure oscillations which is near the backward facing step. This location helps us to record the maximum amplitude of the standing wave. The pressure data is sampled at a rate of 10 kHz.

*Experiments on Aeroacoustic system.* Another fluid mechanical system exhibiting oscillatory instability emerging from a turbulent flow field is an aeroacoustic system. Typically, it consists of orifices located in a duct. Vortices are shed when the turbulent flow passes through the orifice. The schematic of the aeroacoustic experimental setup is shown in Fig. S1b. The aeroacoustic setup consists of a cylindrical chamber, two pipes (lengths: 300 mm and 225 mm respectively), and two circular orifices of diameter 20 mm each, thickness 2.5 mm and separated by a distance of 18 mm. The turbulent flow enters the pipe through the large cylindrical chamber, referred to as the decoupler, which isolates the duct from the upstream pressure

fluctuations. Thus, the pressure at both ends of the duct are maintained at the ambient pressure. The mass flow rate of air is controlled using a mass flow controller (Alicat MCR series) with an uncertainty of ±(0.8% of reading + 0.2% of full scale). The experiments are conducted by increasing the mass flow rate of the air in the duct from 1.633 ± 0.054 g/s to 2.695 ± 0.062 g/s in steps of 0.041 g/s. Correspondingly, the cross-sectional area averaged velocity of the air flow through the orifice varies from 4.24 ± 0.14 m/s to 7.00 ± 0.16 m/s and *Re* varies from 5615 ± 185 to 9270 ± 212. Here, $f$ varies from 484 Hz to 540 Hz as we increase velocity and the corresponding $S_t$ varies from 2.264 ± 0.075 to 1.543 ± 0.035. We measure the pressure fluctuations inside the duct using a pressure field pre-polarized microphone and a preamplifier system (PCB make, model number 378C10, 1 mV/Pa sensitivity and 28.3 Pa resolution) fixed at a distance of 100 mm from the second orifice. The data is sampled at a rate of 10 kHz.

*Experiments on Aeroelastic system.* In a similar manner, we study self-organization in an aeroelastic system. The experimental setup consists of a cantilever beam as shown in Fig. S1c. The right side of the beam is fixed, and the left side of the beam is free. Note that the left end of the beam has a small vertical fin attached to it, akin to a winglet of an aircraft wing. When a jet of air passes along the length of the cantilever from left to right, vortices are shed from the fins. These vortices impart unsteady aerodynamic load to the cantilever. We measure the resulting strain on the cantilever close to the fixed end of the beam (5 mm from the fixed end), using a strain gauge (Micro measurements make, pattern: 125LW, 3% strain range). We increase *Re* from 2384 ± 159 to 4768 ± 111 to capture the transition from low amplitude aperiodic fluctuations to high amplitude oscillatory instability and the corresponding $S_t$ varies from 0.24 ± 0.011 to 0.12 ± 0.003 ($f \sim 60$ Hz). We record the strain data corresponding to the structural vibrations in the system for different values of the control parameter.

**Appendix C: Scaling for transitions from chaos to limit cycle via other types of intermittency.** – In this section, we discuss the results obtained from mathematical models that show the transition from chaos to periodic oscillations via different types of intermittency.

*Type I intermittency.* To study the transition from chaos to periodic oscillations through type I intermittency, we consider the example of a three-dimensional Lorenz system [11]. The system is described as,

$$\begin{aligned} \dot{x} &= \sigma(y - x) \\ \dot{y} &= \rho x - y - xz \\ \dot{z} &= -\beta z + xy \end{aligned} \tag{4}$$

We choose $\sigma = 10$, $\beta = 83$ and $\rho$ as the control parameter which is varied from 175 to 165 in steps of 0.05. In these range of values of the control parameter, the system shows a gradual transition from a chaotic state to a state with finite intervals of regular oscillations amidst intermittent bursts of irregular oscillations and finally to a periodic attractor. The oscillations in the state $z$ are shown in Fig. S2. There is no particular scaling relation observed when we plot the amplitude corresponding to the dominant frequency versus Hurst exponent in a logarithmic scale (Fig. S3a).

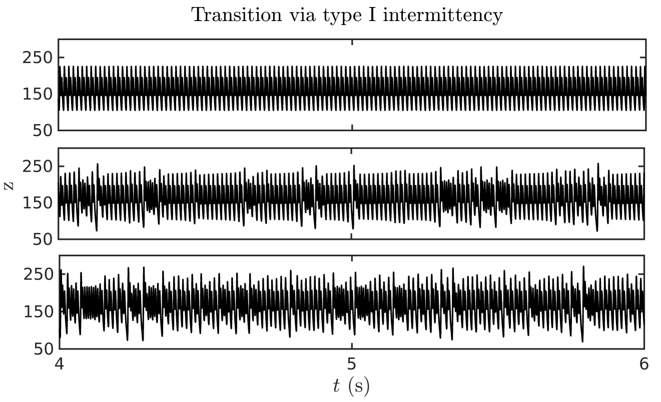


Fig. S2: The oscillations in the state $z$ for selected values of $\rho$ of the Lorenz system. The top figure corresponds to the state of periodic oscillations at $\rho = 165$. We observe type I intermittency (middle figure) around $\rho = 166.5$. The fully chaotic state ($\rho = 172$) is shown in the bottom figure.

We use another example of a generalized Lorenz model [12] to confirm the results for type I intermittency.

$$\begin{aligned} \dot{X} &= \sigma(Y - X) - \omega_0 W \\ \dot{Y} &= rX - Y - XZ \\ \dot{Z} &= -bZ + XY \\ \dot{W} &= \omega_0 - \sigma_m W \end{aligned} \tag{5}$$

This model shows Type I intermittency [12] for the following set of parameters: $r = 256$, $\sigma = 10$, $\sigma_m = 1$, $b = 8/3$. Here $\omega_0$ is the control parameter and is varied between 3.65 and 3.85 in steps of 0.005. The variation of amplitude with Hurst exponent is plotted in Fig. S3b. No particular scaling behaviour is observed during the transition in both Fig. S3a & b.

*Type II intermittency.* The model used to obtain the transition from chaos to limit cycle with type II intermittency is a periodically driven third-order nonlinear oscillator [13]. The following ODE describes the system.

$$\dddot{x} + \eta\ddot{x} + \nu\dot{x} + \mu x + k_1 x^2 + k_2 \dot{x}^2 + k_3 x\dot{x} + k_4 x\ddot{x} + k_5 x^2 \ddot{x} = F cos(\omega t) \tag{6}$$

Figure S4 represents the results after solving the equation (Eq. 6) for the parameter values $F = 0.5$, $\omega = 15$, $\eta = 1$, $\nu = 1.2$, $k_1 = -100$, $k_2 = 120$, $k_3 = 0$, $k_4 = -20$ and $k_5 = 100$. Richetti *et al.* [13] reported this model results showing type II intermittency. They stated that there

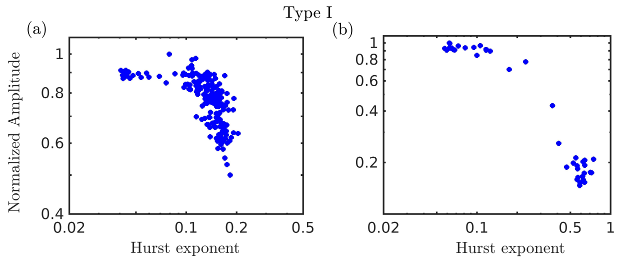


Fig. S3: Variation of the amplitude of the dominant mode with Hurst exponent is plotted in a logarithmic scale for the data generated from models showing type I intermittency. (a), (b) correspond the three dimensional Lorenz model and the generalized Lorenz model respectively. There is no particular scaling observed during the transition in both a & b.

have been no examples identifying type-II intermittency in either real experiments or in simulation studies. Later, an experimental observation of type II intermittency in a coupled nonlinear oscillator has been reported [14]. So, we show only one example for this case.

The parameter is varied to observe the transition from a periodic signal ($\mu = 1.1$) to chaos ($\mu = 1.22$). Further, we observe type II intermittency ($\mu = 1.16$). The amplitude of the dominant mode is plotted with Hurst exponent and shown in Fig. S5. No particular scaling behaviour is observed during the transition via Type II intermittency.

*Type III intermittency.* We study the transition from periodic to chaos through type III intermittency, following the work done by Malasoma *et al.* [15], considering the parametrically excited nonlinear system.

$$\ddot{x}(t) + c\dot{x}(t) + (\omega_0^2 + f cos(\omega t))x(t) + ax^2(t) + bx^3(t) = 0 \quad (7)$$

where, $c$ is the damping coefficient, $a$ and $b$ are quadratic and cubic nonlinearity coefficients, and $\omega_0$ is the natural frequency of the system. Here, $f$ and $\omega$ are the amplitude and the frequency of the sinusoidal parametric excitation. The system is solved for the parameters $c = 0.2$, $\omega_0 = 1$, $a = 1.5$, $b = 0.5$ and $F = 0.85$. We observe periodic oscillations, intermittency and chaos (Fig. S6) at 1.6886, 1.7086 and 1.1682 values of $\omega$ respectively.

Type III intermittency can also be seen in the generalized Lorenz model [12] which is described earlier in the case of type I intermittency. The same model for the following set of values show type III intermittency: $r = 28,\ \sigma = 10,\ \sigma_m = 1,\ b = 8/3$. Here $\omega_0$ is the control parameter and is varied between 2.8 and 5.8 in steps of 0.1. Figure S7 shows the corresponding variation of the amplitude with Hurst exponent for the two models with type III intermittency. We observe that there is no particular scaling relation.

In summary, the models discussed here which exhibit transition from chaos to limit cycle through type I, II & III intermittencies do not seem to follow the scaling behavior observed in the experiments reported in this paper.

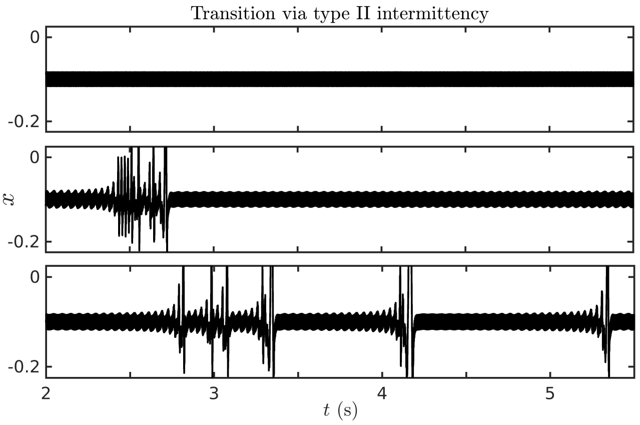


Fig. S4: Time series obtained from a model that shows type II intermittency. The top figure represents periodic oscillations corresponds to $\mu = 1.1$. We observe intermittent transitions to chaos at $\mu = 1.16$ and to a fully chaotic state around $\mu = 1.22$.

## REFERENCES


[1] Kantelhardt J. W., Zschiegner S. A., Koscielny-Bunde E., Havlin S., Bunde A. and Stanley H. E., *Physica A: Statistical Mechanics and its Applications*, **316** (2002) 87.

[2] Mandelbrot B. B. and Wallis J. R., *Water Resources Research*, **5** (1969) 967.

[3] Carbone A., Castelli G. and Stanley H., *Physical Review E*, **69** (2004) 026105.

[4] Ihlen E. A. F. E., *Frontiers in physiology*, **3** (2012) 141.

[5] Kerres B., Nair V., Cronhjort A. and Mihaescu M., *SAE International Journal of Engines*, **9** (2016) 1795.

[6] Nair V. and Sujith R., *Journal of Fluid Mechanics*, **747** (2014) 635.

[7] Nair V., Thampi G. and Sujith R., *Journal of Fluid Mechanics*, **756** (2014) 470.

[8] Unni V. R. and Sujith R., *Journal of Fluid Mechanics*, **784** (2015) 30.

[9] Ghoniem A. F., Park S., Wachsman A., Annaswamy A., Wee D. and Altay H. M., *Proceedings of the Combustion Institute*, **30** (2005) 1783.

[10] Steinberg A. M., Boxx I., Stöhr M., Carter C. D. and Meier W., *Combustion and Flame*, **157** (2010) 2250.

[11] Manneville P. and Pomeau Y., *Physics Letters A*, **75** (1979) 1.

[12] Macek W. M. and Strumik M., *Physical review letters*, **112** (2014) 074502.

[13] Richetti P., Argoul F. and Arneodo A., *Physical Review A*, **34** (1986) 726.

[14] Huang J.-Y. and Kim J.-J., *Physical Review A*, **36** (1987) 1495.

[15] Malasoma J.-M., Lamarque C.-H. and Jezequel L., *Nonlinear Dynamics*, **5** (1994) 153.

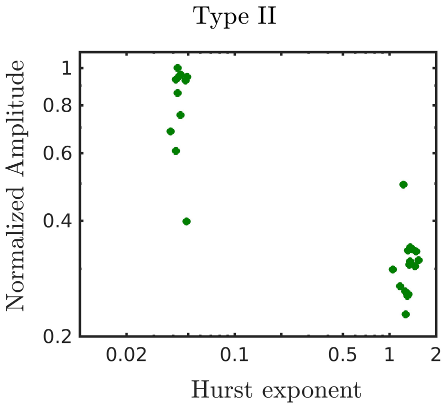


Fig. S5: Variation of the amplitude of the dominant mode with Hurst exponent is plotted in a logarithmic scale for the data generated from model showing type II intermittency. There is no particular scaling observed during the transition.

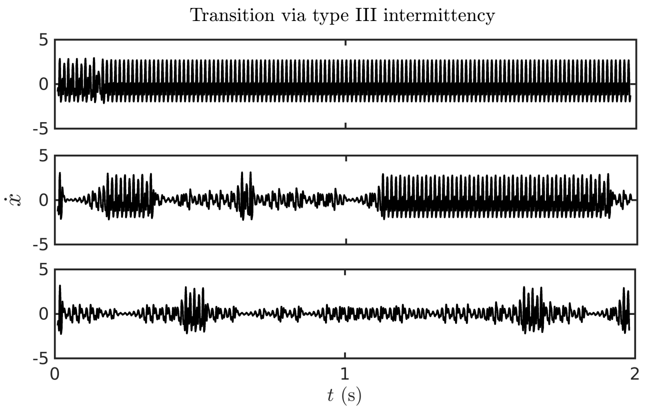


Fig. S6: Time series obtained from a model of a parametrically excited nonlinear system that shows type III intermittency. The figure represents periodic oscillations (top figure) intermittency (middle figure) and a fully chaotic state (bottom figure). We observe a bifurcation happening from periodic oscillations to chaos through type III intermittency.

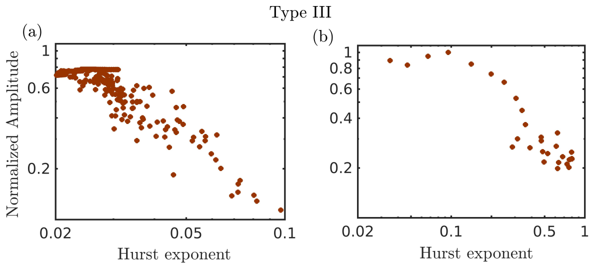


Fig. S7: Variation of the amplitude of the dominant mode with Hurst exponent is plotted in a logarithmic scale for the data generated from models showing type III intermittency. (a) plot of $A$ *vs.* $H$ for a parametrically excited nonlinear system. (b) plot of $A$ *vs.* $H$ for generalized Lorenz model with particular values of the parameter. There is no power law scaling observed during the transition in both the cases.
